# Supplementary material for: Emitter-Vacuum coupling through a leaky nanostructure and the role of dynamics in density of optical states
Source: arXiv:1806.06196 ancillary file (2018-09-11)
Supplement: Supplementary file 1 [file supplementary_Jain.pdf]

# Supplementary Information: Emitter-Vacuum coupling through a leaky metal nanostructure and the role of dynamics in density of optical states

Kritika Jain and Murugesan Venkatapathi*
*Computational and Statistical Physics Laboratory, Indian Institute of Science, Bangalore, 560012*

In the first part of this supplementary, we describe a known method to solve a problem of the modified self-energy of a point dipole source in an inhomogeneous medium that represents nanostructures or a surface. The additional details of experimental and theoretical results presented in the figures follows next.

## I. METHODS

The *total* self-energy[1] of an emitter in presence of the nanostructure is given by[2] :

$$\Sigma(\omega) = \frac{-2\pi q^2\omega}{mc^2}\mathbf{e}_1 \cdot \mathbf{G}(\mathbf{r_o}, \mathbf{r_o}; \omega) \cdot \mathbf{e}_1 - \frac{i\Gamma_o}{2} \quad (1)$$

and the self-energy in equation 1 can be integrated over $\mathbf{e}_1$ for an average over polarization, and also over frequency $\omega$ with the relative spectral density of the free-space emitter as a weight, in case of broad-band emission. Here $q$ is the oscillating charge, $m$ is its mass, and $c$ is speed of light. The decay rate representing the relative density of optical states, is given by $\Gamma = -2\Im(\Sigma)$, where $\Sigma$ is the modified self-energy in presence of the nanostructure. $\Gamma_0^r$ and $\Gamma_0^{nr}$ are known radiative and non-radiative decay rates of the isolated emitter adding to $\Gamma_o$. Here $\Gamma_0^r = \frac{2\sqrt{\epsilon_o}\mu^2k^3}{3\hbar}$ and $\mu$ is the electric dipole moment of the emitter; $k$, $\epsilon$ and $\hbar$ are the wave number, free-space permittivity and reduced Planck's constant. Thus it is convenient for evaluations to normalize all self-energy components by $\Gamma_0^r$. Note that a dipole oscillator with energy of one quantum represents the emitter as a two-level system in this weak vacuum-coupling regime. In all cases presented in this work, $\frac{|\Re(\Sigma)|}{\omega} < 0.01$, and the rotating wave approximation for the energy shifts is useful.

Consider an emitter located at $\mathbf{r_o}$ interacting with a nanostructure or inhomogeneous matter in general, where the permittivity is a function of $\mathbf{r}$. The dyadic Green function describing this interaction in a medium of isotropic permitivitty $\epsilon(r)$ is the solution of:

$$\nabla \times \nabla \times \mathbf{G}(\mathbf{r}, \mathbf{r_o}; \omega) - \epsilon(r;\omega)k^2\mathbf{G}(\mathbf{r}, \mathbf{r_o}; \omega) = \mathbf{I}\delta(\mathbf{r} - \mathbf{r_o}). \quad (2)$$

where $\mathbf{I}$ is a unit dyad, the wave number $k = \frac{\omega}{c}$, and $\delta(\mathbf{r} - \mathbf{r_o})$ represents a point source.

* murugesh@iisc.ac.in

The above equation has no analytical solutions in general, and a quasi-static solution in the long wavelength limit has been typically preferred. But this may result in significant errors, especially in its underestimation of non-radiative decay rates in metal nanostructures. Hence, one has to resort to more computationally intensive full-wave approaches to include retardation for finite wavelengths. We used the more efficient Sommerfeld integral solutions [3–5] to compute the retarded wave image-dyadic for a surface in the near-field (for the results in figure 5). A different approach used for the metal nano spheres discussed in figures 1 - 4, is discretization of the nanostructure into very small dipole granules. These two methods to evaluate the dyadic Green tensors for the corresponding problems are described separately. In addition we present here (in figure S2) evaluations using the quasi-static approximations for a surface which are more widely used. We also present the predictions of enhancements for the metal nano spheres using the single dipole approximation (figures S5 and S6). This is to confirm that the more intensive computational approach adds only to the non-radiative contributions of the higher order modes as expected, and indeed does not alter the conclusions of this work.

### A. Self-interaction dyads for emitters near arbitrary nanostructures

First we perform a discretization of the nanostructure into very small dipole granules, where interaction between any two dipole granules $i, j$ is well approximated by the point-dipole dyadic:

$$\mathbf{G}(\mathbf{r_i}, \mathbf{r_j}; \omega) = (\mathbf{I} + \frac{\nabla\nabla}{k^2})g(\|\mathbf{r_i} - \mathbf{r_j}\|) \quad (3)$$

where $g(r) = \frac{e^{ikr}}{4\pi r}$ The green dyadic for estimating the modified self-interaction of an emitter in presence of the nanostructure is given by[6]:

$$\mathbf{G}(\mathbf{r_o}, \mathbf{r_o}; \omega) = -\bar{G}_{ob} \cdot \bar{G}_{bb}^{-1} \cdot \bar{G}_{ob}^T. \quad (4)$$

where $\bar{G}_{bb}$ is $3m \times 3m$ matrix that represents interaction among $m$ dipole granules in the nanostructure and $\bar{G}_{ob}$ is a $3 \times 3m$ matrix that represents interaction between the emitter and each dipole granule of the nanostructure ($m$ is in the order of $10^3 - 10^4$ for results presented in this work). Both these matrices are constructed using the $3 \times 3$ point-dipole Green dyads in equation (3) for

any two entities at $r_j, r_i$. The dipolar components can be factored from the total values, by an evaluation using a single dipole with the volume polarizability of the body. A decomposition of the metallic component $\Gamma$ into its radiative and non-radiative components $\Gamma^r$ and $\Gamma^{nr}$ in case of an arbitrary structure consisting dipole granules, involves factoring out the contribution of real and imaginary parts of permittivity of granules to the dyad $\mathbf{G}$, and this was shown elsewhere [6].

### B. Self-interaction dyads for emitters near surfaces

In case of the surface models used here, $\mathbf{G}$ is given by[4]:

$$\mathbf{G} = \mathbf{S} + \frac{k_2^2}{\epsilon_2}\frac{k_1^2 - k_2^2}{k_1^2 + k_2^2}\mathbf{G}^I \tag{5}$$

where $\mathbf{G}^I$ is image Green dyadic and the components of $\mathbf{S}$ matrix are given by Sommerfeld integrals. The Sommerfeld integrals are computed numerically using a method developed by Lager and Lytle [3], where $k_1$ and $k_2$ are the wave numbers for the surrounding and surface respectively.

$$\mathbf{G}^I = -\mathbf{G} \cdot \mathbf{I}_R \tag{6}$$

where $\mathbf{I}_R$ is the reflection dyad of the surface with normal as the Z-axis, given by $\mathbf{e}_x\mathbf{e}_x + \mathbf{e}_y\mathbf{e}_y - \mathbf{e}_z\mathbf{e}_z$.

In case of Sommerfeld model, note that we are restricted to an integral over a distribution of image-dipolar sources with corresponding phases [5]. Decomposition of $\mathbf{G}$ into its radiative ($\mathbf{G}^r$) and non-radiative parts ($\mathbf{G}^{nr}$) use the fact that imaginary part of polarizability of image dipole denotes absorption and its real part denotes scattering.

In the front factor of R.H.S of equation (5), Fresnel reflection coefficient (polarizability of the image dipole) can be written as :

$$\frac{k_1^2 - k_2^2}{k_1^2 + k_2^2} = \frac{\epsilon_r - 1}{\epsilon_r + 1} \tag{7}$$

where $\epsilon_r$ is permittivity of metal surface with respect to surrounding medium.

$$\mathbf{G}^r = \mathbf{S} + \frac{k_2^2}{\epsilon_2}\Re\left(\frac{k_1^2 - k_2^2}{k_1^2 + k_2^2}\right)\mathbf{G}^I \tag{8}$$

$$\mathbf{G}^{nr} = \frac{k_2^2}{\epsilon_2}\Im\left(\frac{k_1^2 - k_2^2}{k_1^2 + k_2^2}\right)\mathbf{G}^I \tag{9}$$

Hence,

$$\Gamma^{total} = -2\Im\left(\frac{-2\pi q^2\omega}{mc^2}\mathbf{e}_1 \cdot \mathbf{G} \cdot \mathbf{e}_1\right) + \Gamma_0 \tag{10}$$

$$\Gamma^r = -2\Im\left(\frac{-2\pi q^2\omega}{mc^2}\mathbf{e}_1 \cdot \mathbf{G^r} \cdot \mathbf{e}_1\right) + \Gamma_0^r \tag{11}$$

$$\Gamma^{nr} = \Gamma^{total} - \Gamma^r \tag{12}$$

The contribution of $\mathbf{S}$ to $\Gamma^r$ are small due to its small imaginary values in the self-interaction problem. But it has a large real part that contributes significantly to the real part of the self-energy i.e. the energy shifts. Thus predictions of these retarded wave evaluations are marginally different from the quasi-static approximation below.

In the quasi-static case :

$$\mathbf{G} = \frac{k_1^2 - k_2^2}{k_1^2 + k_2^2}\mathbf{G}^I \tag{13}$$

where $\mathbf{G}^I$ is purely real, unlike the the above retarded wave self-interaction dyad. Further decomposition of $\mathbf{G}$ and $\Gamma^{total}$ into $\Gamma^r$ and $\Gamma^{nr}$ is similar to the Sommerfeld model case. Here, the imaginary part of the Fresnel reflection coefficient represents the imaginary part of the polarizability of image dipole, and thus contributes to $\Gamma^{nr}$. The real part of Fresnel coefficient contributes to the energy shifts. Thus $\Gamma^{total} = \Gamma^{nr} + \Gamma_0^r + \Gamma_0^{nr}$ and $\Gamma^r = \Gamma_0^r$ i.e contribution of metal surface to the radiative decay is null in the quasi-static case.

## II. RESULTS

In this part of supplementary, we describe the additional details of experimental results presented in the five figures of the paper. These experimental enhancements observed were compared with both relative quantum efficiency $Q$ and relative power of emission $Q\Gamma^r$, with respect to the emitters not interacting with metal nanostructures. The former represents the increase in probability of radiative decay of the excited emitter, while the latter also includes increase in ground-state population for emitters that can be excited continuously.

### A. Figure 1

Experimental data points (green triangles) in Figure 1 are from ref. [7]. In their experiment, they used gold nanoparticles of diameter 10 nm (i.e. radius 5 nm). They were coated with the bi-polymer PAH/PSS ($\epsilon_r = 2.5$). Then Cypate, used as fluorophore, was placed on these polymer-coated gold nanoparticles. The emission peak of Cypate was at 830 nm and while the resonance peak of gold nanoparticles in free-space is around 520 nm, it red-shifts significantly due to the polymer coating. The quantum efficiency of Cypate was 0.012. We consider all these parameters in our theoretical evaluations for a comparison with their experimental data. The three experimental data points $(2.5, 5)$, $(4.5, 17)$, $(6.5, 10)$ are from figure 9 of that paper [7].

### B. Figures 2 and 3

Experimental data points in Figures 2 and 3 are from ref no. [8]. In this experiment, they studied 13 nm diameter (6.5 nm radius) gold nanoparticles and fabricated metal core-polymer shell capsules with two different dyes, fluorescein ($FITC$) and lissamine rhodamine B ($LISS$), situated at various distances from the gold core. For FITC, mean distances between the surface of the Au core and the fluorescent layers were 1.5 ± 0.3 nm, 4.0 ± 0.5 nm, and 7.9 ± 0.7 nm; for LISS, the corresponding distances were 1.8 ± 0.3 nm, 3.9 ± 0.5 nm, and 7.7 ± 0.6 nm. Emission wavelengths of both the dyes are borrowed from Figure 4 in ref. [8]; for FITC it is around 520 nm and for LISS it is around 580 nm. We consider all these parameters in our theoretical predictions and compare with their experimental data. In theoretical predictions, intrinsic quantum efficiency ($Q_o$) used for fluorescein was 1 and for lissamine rhodamine B was 0.37 as provided in Table 1 of the paper [8]. The refractive index of polymer layer used was 1.42.

Figure 2 is for the dye FITC in which green triangles show relative fluorescence intensity. These data points $(1.8, 0.11)$, $(4, 0.24)$, $(7.9, 0.29)$ are from Figure 5 and table 2 in the paper [8]. Figure 3 is for the dye LISS in which green triangles show relative fluorescence intensity. These data points $(1.8, 0.2)$, $(3.9, 0.45)$, $(7.7, 0.6)$ are from figure 5 [8]. Here experiments exhibit more quenching at large distances and compared to fluorescein, lissamine appears to be particularly affected by the incorporation in the layer-by-layer polymer capsules which can be inferred by Table 1 [8]. It may be that LISS is more sensitive to electron transfer quenching by amino groups than FITC. In our computation, we ignored electron transfer quenching due to polymer layers. Thus both the conventional and proposed theoretical predictions may have marginally overestimated the emission in figure 3.

### C. Figure 4

Experimental data points in left section of Figure 4 [9] represent monolayers with radii of gold nanoparticles approximately 1.75 nm. Distances between the surface of nanoparticle to emitter for different number ratios ($N_{CdSe} : N_{Au}$) are in Table 1 of that paper [9]. Green triangles (left side) in Figure 4 of our paper are from Fig 4 in ref.[9] where PL enhancements factors were plotted for different samples using two methods. All data points are in good agreement with proposed theory while conventional theory shows strong quenching. Right section of figure 4 represents experimental data [10] from block-copolymer (BCP) templates which form cylindrical phases in bulk and in thin films and quantum dots were incorporated inside those cylindrical templates. The diameter of cylinder and inter-cylinder spacing were approximately 40 nm and 100 nm respectively [11]. Au-NPs were randomly distributed outside the cylinders. Schematic representation of hybrid films in the polymer template showing the dispersion of CdSe quantum dots in P4VP block and Au nanoparticles in PS block is given in Figure 1 of that paper [10]. The estimated distance between Au-NPs and center of the nearest P4VP cylinder was approximately 35-40 nm. They used Au-NPs of mean diameters 2 nm and 5 nm and CdSe quantum dots with average diameters 4 nm and 6 nm. We simulated our results for single Au-NP of diameter 5 nm interacting with a single dipole emitter (quantum dot) at different surface to dipole distances. Note that the smallest Au-NPs of 2 nm used in their experiments may have accumulated into larger nanoparticles of mean sizes 20 nm [11] and thus not relevant for our study. We assumed initial quantum efficiency of emitter to be 0.05 as measured (table II in ref. [10]). Four points $(12.5, 2.56)$, $(12.5, 1.69)$, $(12.5, 1.9)$, and $(12.5, 1.38)$ represented by green triangles on right side in Figure 4 of our paper are from Figure 3 of Ref. [10] where fluorescence of four different samples of quantum dots doped with 5 nm gold nanoparticles and bare quantum dots was presented. Our results represent a surface to emitter distance of 12.5 nm i.e. the mean surface - surface distance of the closest quantum dot (at the surface of the cylinders) to Au-NPs according to that geometry. But on balance, we ignore the effect of other Au-NPs possibly at larger distances, thus reflecting the experiments reasonably.

### D. Figures 5, S1 and S2

In our evaluation for SERS plots, we used the Sommerfeld integrals [3–5] to compute dyadic green's function in presence of the surface. The subsequent evaluation of self-energy, decay rates was described in section 1 of this supplementary. To account for the spatial variation of near field enhancement, $(E_{local}/E_o)^2$, due to features on a surface, we evaluated $\sqrt{(E_{local}/E_o)^4}$ where

$$\frac{E_{local}^4}{E_o^4} = 10^8 * (1 + \frac{h}{a})^{-10} \tag{14}$$

where $h$ is the distance between emitter and the metal surface, and $a$ is average size of features on the surface i.e radius of nano islands in this case. The relative intensity i.e. $(1 + \frac{h}{a})^{-10}$ [12, 13] is multiplied by a factor of $10^8$, as the maximum $(E_{local}/E_o)^2$ evaluated or observed so far for various structures has been up to $10^4$ [14–16].

Emission wavelength of emitter was 550 nm with a $Q_o$ of 0.33 without loss of generality of the plot, as variations in the enhancements with $Q_o$ are relatively small. We used a silver surface and refractive index of surrounding medium was 3.5 to tune the surface plasmon resonance to 550 nm. Silver has a permitivitty of $-12.93 + 0.428i$ at 550 nm, and with surrounding medium of refractive index 3.5, the relative permittivity reduces to $-1.056 + 0.035i$ satisfying Fröhlich condition for surface plasmon resonance.

In Figure 5, solid and dotted lines show results of proposed theory and conventional theory respectively for 10 nm (diameter) nano islands. Error bars show deviation of the results on varying size of nano islands from 2 nm to 50 nm. The upper end of error bars represent results for nano islands of 50 nm size while lower ends represent 2 nm nano islands. Another figure S1 below is enlarged to highlight those results for short range. Green triangles are from experiments done by others [17–22]. Distance dependent measurements are taken from Figures 5, 6 and 7 in Ref.[18] and Figures 1 and 2 in Ref.[17]. In Figure 2 of Ref.[17], normalized SERS enhancement factor was provided and '1' there represents a gain of 3000 (the largest gain in figure 1 thereof). Other experimental measurements without any spacer between SERS substrate and emitter are plotted at a near-zero distance [19–22].

For the results in Figure S2, we used quasi-static approximation i.e., retardation is neglected. We used image dipole theory to compute dyadic green's function [23]. The subsequent evaluation of self-energy decomposition into radiative and non-radiative parts was described in section 1 of this supplementary. All other parameters are the same as of figure 5. In the quasi-static limit, $\Gamma^{nr}$ is underestimated and hence quantum efficiency is overestimated; as a result the black line in figure S1 falls above the experiments. Also, in conventional theory, power and $Q\frac{E^2}{E_o^2}$ coincide in the quasi-static limit as the enhancement in radiative rates due to the surface is negligible in this case.

### E. Figure S3

Figure S3 is similar to Figure 5 (SERS results using sommerfeld integral method). Here we modeled a gold surface with a refractive index of surrounding medium as 2. Gold has a permitivitty of $-5.93 + 2.097i$ at 550 nm, and the relative permittivity reduces to $-1.48 + 0.52i$. Hence, figure S3 is depicting off-resonance SERS results.

### F. Figure S4

Experimental data points in Figure S4 are from Ref no. [24]. In Figure 4 of their paper, radiative and non-radiative decay rates were plotted separately. They were added to get the $\Gamma_{total}$ here and are further normalized by $\Gamma_0^r$ $(0.21 * 10^9 s^{-1})$ in the plot. Typically, the decomposition of the total decay rate into radiative and non-radiative parts can have variations depending on the instrument gains and methods used. But the total decay rates are expected to be robust. A notable anomaly in this experimental observation[24] was that the total decay rate of emitter increased by only a factor of 2, even when the size of the gold nanoparticles increased from 2 to 60 nm. Note that the emitters were supposed to be separated by a distance of 1 nm from the surface of a nanoparticle of any size; this is in general a challenging requirement in experiments. Using theoretical evaluations, we estimate that the under-reported changes in decays were probably due to a varying distance from nanoparticles of different sizes as shown in the figure S3. As the size of nanoparticles increased so may be did the distance of separation.

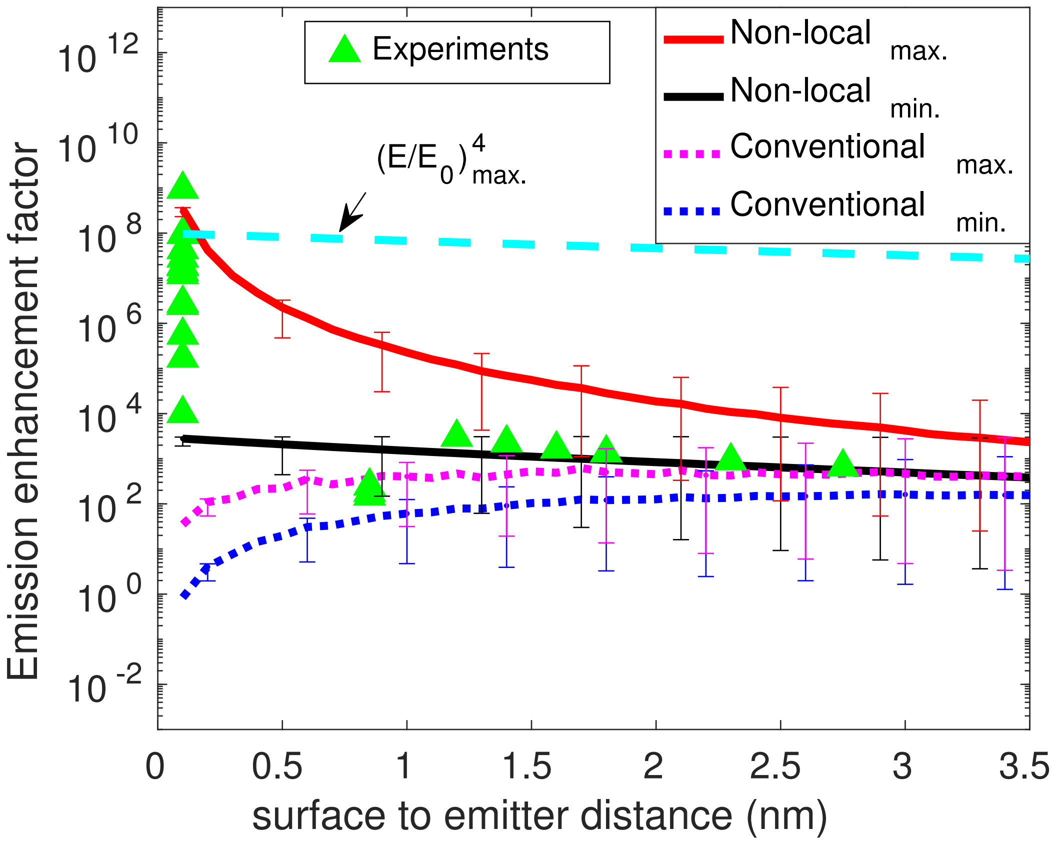


FIG. 1. Short-distance comparison of (full retarded wave) theoretical and experimental SERS results in figure 5: The minimum and maximum gains predicted are given by effective values of quantum efficiency $Q\frac{E^2}{E_o^2}$ and power radiated $Q\Gamma^r\frac{E^2}{E_o^2}$, normalized by the values of isolated emitter; note *log*-scale in Y-axis. Relative $\epsilon = -1.05 + 0.035i$ for the half-space forming the surface. Error bars placed alternately for conventional and non-local theories reflect variations in predictions using near-field enhancements by 2 to 50 nm size features on the metallic surface, where the lines represent a 10 nm feature.

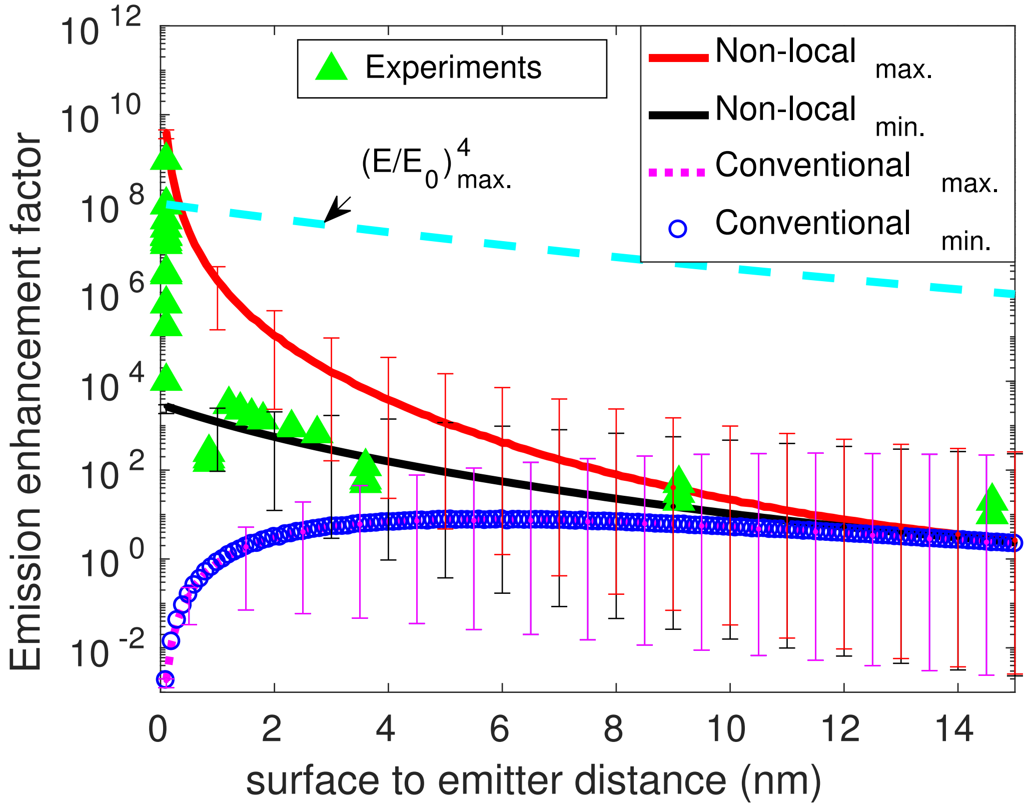


FIG. 2. Comparison of (quasi-static) theoretical and experimental SERS results: The minimum and maximum gains predicted are given by effective values of quantum efficiency $Q\frac{E^2}{E_o^2}$ and power radiated $Q\Gamma^r\frac{E^2}{E_o^2}$, normalized by the values of isolated emitter; note *log*-scale in Y-axis. Relative $\epsilon = -1.05 + 0.035i$ for the half-space forming the surface. Error bars placed alternately for conventional and non-local theories reflect variations in predictions using near-field enhancements by 2 to 50 nm size features on the metallic surface, where the lines represent a 10 nm feature.

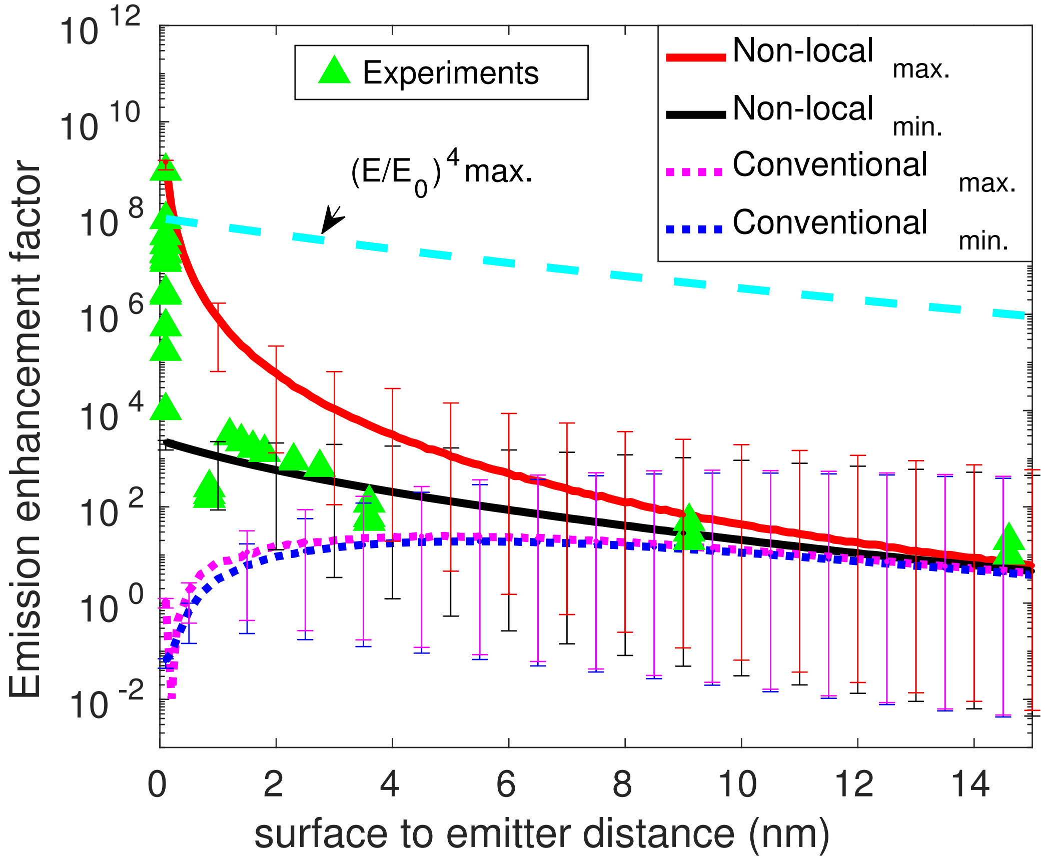


FIG. 3. Comparison of (full retarded wave) theoretical and experimental SERS results: The minimum and maximum gains predicted are given by effective values of quantum efficiency $Q\frac{E^2}{E_o^2}$ and power radiated $Q\Gamma^r\frac{E^2}{E_o^2}$, normalized by the values of isolated emitter; note *log*-scale in Y-axis. Relative $\epsilon = -1.48 + 0.524i$ for the half-space forming the surface. Error bars placed alternately for conventional and non-local theories reflect variations in predictions using near-field enhancements by 2 to 50 nm size features on the metallic surface, where the lines represent a 10 nm feature.

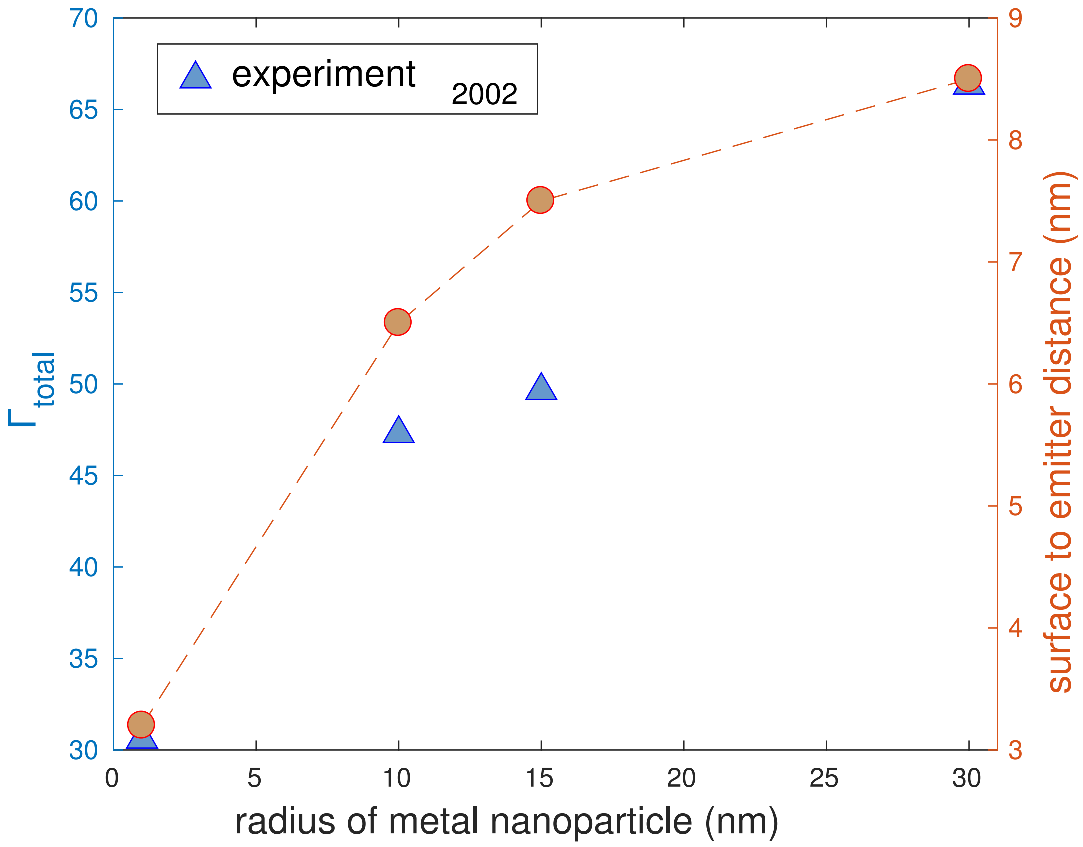


FIG. 4. The theoretical predictions of the separations are marked on the Y-axis on the right, for the observed decay rates reported[24]. Note experiments were designed for the emitter to be separated from the surface of the metal nanoparticle by a distance of 1 nm, in all cases. Here the observed $\Gamma_{total}$ marked on the Y-axis on the left, are normalized by radiative decay rate of the isolated emitter i.e. $\Gamma_0^r$.

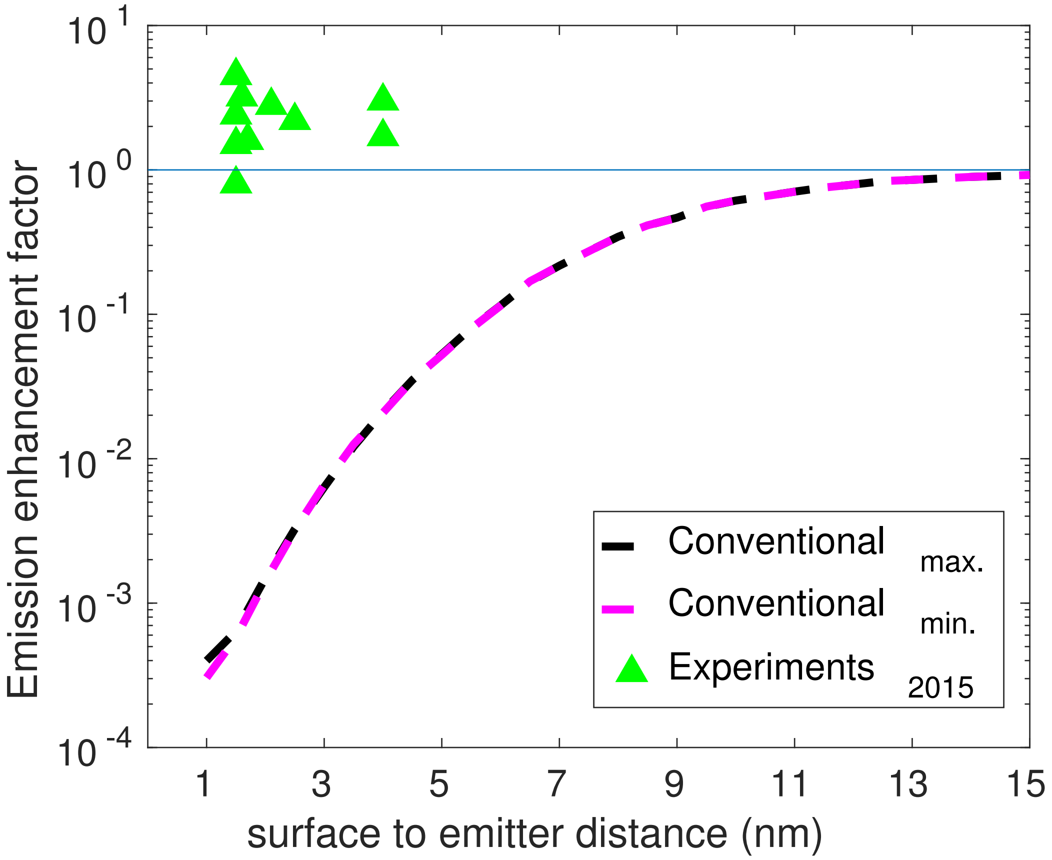


FIG. 5. Comparison of theoretical (single dipole approximation of nano sphere) and experimental results: The minimum and maximum gains predicted are given by quantum efficiency $Q$ and power radiated $Q\Gamma^r$, normalized by the values of isolated emitter; note *log*-scale in Y-axis. Experimental data [9] is for gold nanoparticles of radius 1.75 nm and the peak emission wavelength is 560 nm.

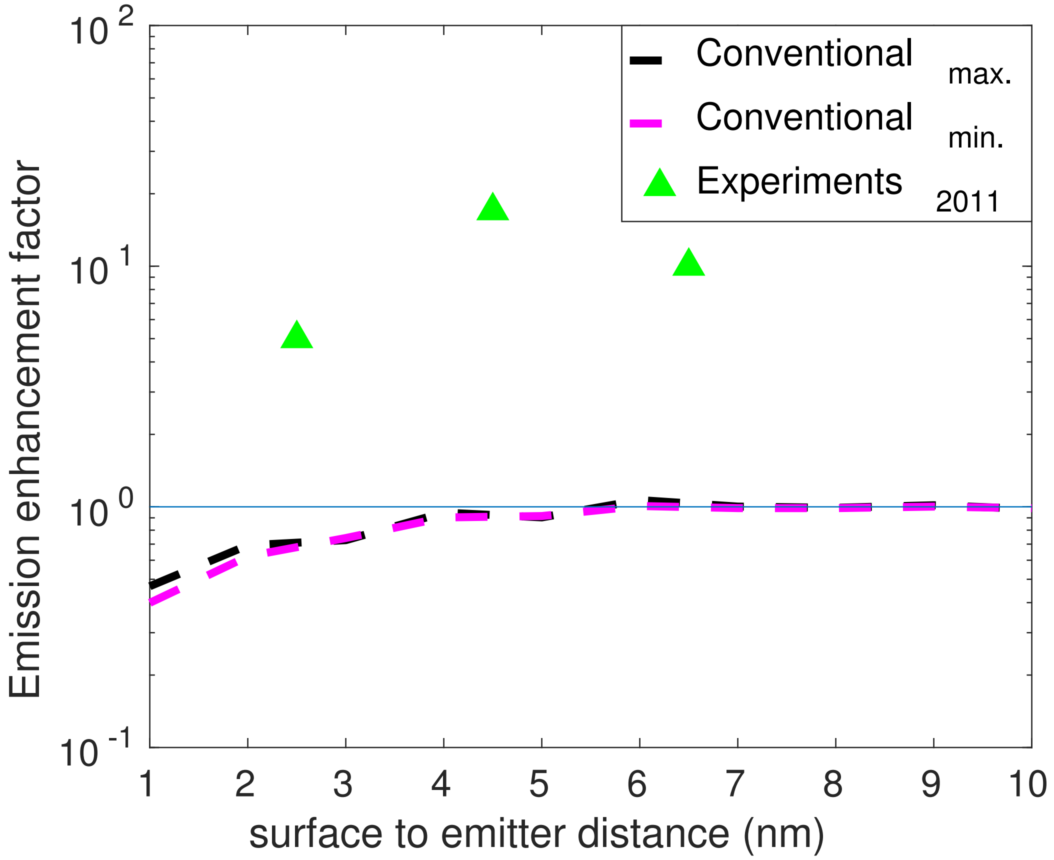


FIG. 6. Comparison of theoretical (single dipole approximation of nano sphere) and experimental results: The minimum and maximum gains predicted are given by quantum efficiency $Q$ and power radiated $Q\Gamma^r$, normalized by the values of isolated emitter; note *log*-scale in Y-axis. Experimental data[7] is for a gold nanoparticle of radius 5 nm coated with a bi-polymer and the peak emission wavelength was 830 nm.

[1] A. Barut and J. Dowling, Phys. Rev. A **36**, 649 (1987).

[2] V. N. Pustovit and T. V. Shahbazyan, Phys. Rev. Lett. **102**, 077401 (2009).

[3] R. J. Lytle and D. L. Lager, Tech. Rep., Lawrence Livermore Laboratories (1974).

[4] R. Schmehl, B. M. Nebeker, and E. D. Hirleman, J. Opt. Soc. Am. A **14**, 3026 (1997).

[5] I. Arun and M. Venkatapathi, Appl. Numer. Math. **106**, 79 (2016).

[6] M. Venkatapathi, J. Opt. Soc. Am. B **31**, 3153 (2014).

[7] K. A. Kang, J. Wang, J. B. Jasinski, and S. Achilefu, J. Nanobiotechnol. **9**, 16 (2011).

[8] G. Schneider, G. Decher, N. Nerambourg, R. Praho, M. H. Werts, and M. Blanchard-Desce, Nano Lett. **6**, 530 (2006).

[9] M. Praveena, A. Mukherjee, M. Venkatapathi, and J. Basu, Phys. Rev. B **92**, 235403 (2015).

[10] M. Haridas, J. Basu, A. Tiwari, and M. Venkatapathi, J. Appl. Phys. **114**, 064305 (2013).

[11] M. Haridas and J. Basu, Nanotechnol. **21**, 415202 (2010).

[12] B. Kennedy, S. Spaeth, M. Dickey, and K. Carron, J. Phys. Chem. B **103**, 3640 (1999).

[13] J. A. Dieringer, A. D. McFarland, N. C. Shah, D. A. Stuart, A. V. Whitney, C. R. Yonzon, M. A. Young, X. Zhang, and R. P. Van Duyne, Faraday Discussions **132**, 9 (2006).

[14] Y. Huang, L. Ma, M. Hou, J. Li, Z. Xie, and Z. Zhang, Scientific reports **6**, 30011 (2016).

[15] G. Pellegrini, M. Celebrano, M. Finazzi, and P. Biagioni, The Journal of Physical Chemistry C **120**, 26021 (2016).

[16] G. C. Schatz, M. A. Young, and R. P. Van Duyne, in *Surface-enhanced Raman scattering* (Springer, 2006), pp. 19–45.

[17] Q. Ye, J. Fang, and L. Sun, J. Phys. Chem. B **101**, 8221 (1997).

[18] G. Kovacs, R. Loutfy, P. Vincett, C. Jennings, and R. Aroca, Langmuir **2**, 689 (1986).

[19] D. Wang, W. Zhu, M. D. Best, J. P. Camden, and K. B. Crozier, Sci. Rep. **3**, 2867 (2013).

[20] A. M. Gabudean, M. Focsan, and S. Astilean, J. Phys. Chem. C **116**, 12240 (2012).

[21] V. Ivanov, N. Todorov, L. Petrov, T. Ritacco, M. Giocondo, and E. Vlakhov, in *J. Phys.: Conference Series* (IOP Publishing, 2016), vol. 764, p. 012023.

[22] A. D. McFarland, M. A. Young, J. A. Dieringer, and R. P. Van Duyne, J. Phys. Chem. B **109**, 11279 (2005).

[23] L. Novotny and B. Hecht, *Principles of nano-optics* (Cambridge university press, 2012).

[24] E. Dulkeith, A. Morteani, T. Niedereichholz, T. Klar, J. Feldmann, S. Levi, F. Van Veggel, D. Reinhoudt, M. Möller, and D. Gittins, Phys. Rev. Lett. **89**, 203002 (2002).
